# Supplementary material for: Structured learning of rigid-body dynamics: A survey and unified view from a robotics perspective
Source: arXiv:2012.06250 source file (2021-04-16)
Supplement: Supplementary file 1 [file section5_appendix.tex]

\appendix

\section{- Multivariate Gaussian Processes} \label{sec:appendix_gp}
A GP $f(x)$ is any distribution over functions such that finite sets of function values $f(x_1), f(x_2), ... ,f(x_N)$ are jointly Gaussian distributed \cite[Chapter 2]{williams2006gaussian}.

A multivariate GP $f(x) \sim \mathcal{GP}(\mathbf{m}(x), \mathbf{k}(x,x'))$, also often referred to as multi-output or corregionalized GP \cite{alvarez2011kernels} is defined by its vector-valued mean function
\begin{equation}
    \E[f(x)] = \mathbf{m}(x),
\end{equation}
with $\mathbf{m}(x) : \mathbb{R}^{D} \to \mathbb{R}^{n}$ and matrix-valued kernel function
\begin{equation}
    \text{Cov} [f(x),f(x')] = \mathbf{k}(x,x')
\end{equation}
% \text{Cov} [f(x),f(x')] = \E\Big[\big(f(x)-\mu(x)\big) \big(f(x')-\mu(x')\big)^\transp\Big] = k(x,x')
with $\mathbf{k}(x,x') : \mathbb{R}^{D \times D} \to \mathbb{R}^{n \times n}$. Note that the kernel itself is a block-matrix defining the covariance between the individual process components, \eg in the case of $f \in \mathbb{R}^2$ we have
\begin{equation}
\mathbf{k}(x,x') =
\left(
    \begin{array}{cc}
         \text{Cov} [f_1(x),f_1(x')] & \text{Cov} [f_1(x),f_2(x')]  \\
         \text{Cov} [f_2(x),f_1(x')] &  \text{Cov} [f_2(x),f_2(x')]
    \end{array} \right) =
    \left(
    \begin{array}{cc}
         k_{1,1}(x,x') & k_{1,2}(x,x') \\
         k_{1,2}(x,x') & k_{2,2}(x,x') 
    \end{array} \right).
\end{equation}
Oftentimes we are interested in predicting a process at a stack of inputs $[x^{*}_1, x^{*}_2, ... , x^{*}_{N'}] := X^{*}$ using observations at a stack of input vectors $[x_1, x_2, ... , x_N] := X$. If the observations are modelled as $\hat{f}(x) = f(x) + \epsilon_{\hat{f}}$ with $\epsilon_{\hat{f}} \sim \mathcal{N}(0,\Sigma_{\hat{f}})$, then predictions of $f(X^{*})$ are  made via the formula for Gaussian conditionals
\begin{align}
f(X^{*}) \mid \hat{f}(X), X, \mathbf{m}(\cdot), \mathbf{k}(\cdot,\cdot) \sim \mathcal{N}\Big(\mu(X^{*})+\KsT\big(\K + \Sigma_{\hat{f}}\big)^{-1}\big[\hat{f}(X)-\mu(X)\big], \nonumber\\
 \Kss-\KsT\big(\K + \Sigma_{\hat{f}} \big)^{-1} \Ks\Big),
\end{align}
where we use for the Gram matrices whose $i, j$-th block-matrix is given by $\mathbf{k}(x_i, x_j)$, the following notation
\begin{align}
\K &=\mathbf{k}(X, X), \\
\Ks &=\mathbf{k}(X, X^{*}), \\
\Kss &=\mathbf{k}(X^{*}, X^{*}).
\end{align}
